# Supplementary material for: The Rashomon Importance Distribution: Getting RID of Unstable, Single Model-based Variable Importance
Source: arXiv:2309.13775 source file (2024-04-01)
Supplement: Supplementary file 1 [file ecr_ccr_proof.tex]

%%% NOT READY FOR REVIEW 

\begin{corollary}
    % Let $\varepsilon_H, \delta > 0$. 
    The $\alpha$-central credible region ($CCR$) describes the range of values in  which $100\cdot(1-\alpha)\%$ of a distribution's central mass lies. In a univariate distribution, this quantity can be found using the $\frac{\alpha}{2}$ and $(1 - \frac{\alpha}{2})$ quantiles. The $\tau$-th quantile of a random variable $A$ is any value of $k$ such that $\mathbb{P}(A \leq k) = \tau.$ We define a new robustness region, the estimated coverage region ($ECR$): given $\varepsilon_E > 0,$ let $\tau_{low} = \frac{\alpha}{2} - 2\varepsilon_E$ and $\tau_{up} = 1 - \frac{\alpha}{2} + 2\varepsilon_E.$ Then, define 
    \begin{align*}
        ECR = \left(\hat{Q}_{\tau_{low}}, \hat{Q}_{\tau_{up}} \right),
    \end{align*}
    where $Q_{\widehat{\ourvi}}(\tau)$ is the $\tau$-th quantile of $\widehat{\ourvi}$.
    
    With high probability, $ECR$ is guaranteed to cover $\ourvi's$ $CCR$ using $\widehat{\ourvi}$. Specifically, with probability $1 - \delta,$
    \begin{align*}
        CCR \subset ECR
    \end{align*}
    with $B \geq \frac{1}{2\varepsilon^2}\ln\left( \frac{8}{\delta} \right)$ bootstrap iterations.
    
    % Let $Q_{\frac{\alpha/2}}$ and $Q_{1 - \frac{\alpha}{2}}$ represent the $\alpha\%-$central credible region in $\ourvi.$ These are the $\frac{\alpha}{2}$ and $100 - \frac{\alpha}{2}$ percentiles in $\ourvi.$ 
    
    % Given quantiles of interest $t_{\text{low}}$ and $t_{\text{up}}$ such that $t_{\text{low}} < t_{\text{up}}$, let $\tau_{\text{low}}:= t_{\text{low}} - 2\varepsilon_H $ and $\tau_{\text{up}}:= t_{\text{up}} + 2\varepsilon_H $. Let $CCR(t_{\text{low}}, t_{\text{high}}):=\mathbb{P}(\ourvi \leq Q_{\ourvi}(t_{\text{low}}) ), \mathbb{P}(\ourvi \leq Q_{\ourvi}(t_{\text{up}}) )$ denote the region between the $t_{\text{low}}$-th quantile and the $t_{\text{up}}$-th quantile of $\ourvi$, and let $\widehat{CCR}(\tau_{\text{low}}, \tau_{\text{up}}):=\mathbb{P}(\widehat{\ourvi} \leq Q_{\widehat{\ourvi}}(\tau_{\text{low}}) ), \mathbb{P}(\widehat{\ourvi} \leq Q_{\widehat{\ourvi}}(t_{\text{up}}) )$ denote the region between the $\tau_{\text{low}}$-th quantile and the $\tau_{\text{up}}$-th quantile of $\widehat{\ourvi}$.
%     Then, with probability at least $1 - 4\delta$,
%     \begin{align*}
%         \left(\mathbb{P}(\ourvi \leq Q_{\ourvi}(t_{\text{low}}) ), \mathbb{P}(\ourvi \leq Q_{\ourvi}(t_{\text{up}}) )\right)\subseteq \left(\mathbb{P}(\widehat{\ourvi} \leq Q_{\widehat{\ourvi}}(\tau_{\text{low}}) ), \mathbb{P}(\widehat{\ourvi} \leq Q_{\widehat{\ourvi}}(\tau_{\text{up}}) )\right)
%     \end{align*}
% with $B \geq \frac{\ln\left( \frac{1 - \delta}{2} \right)}{-2\varepsilon_H^2}$ iterations.
\end{corollary}
\begin{proof}

    Let $t_{\text{low}}, t_{\text{up}} \in (0, 1)$ such that $t_{\text{low}} < t_{\text{up}}$, and let $\varepsilon_H, \delta > 0$. Let $Q_{\widehat{\ourvi}}(\tau)$ denote the $\tau$-th quantile of $\widehat{\ourvi}$ and $Q_{\ourvi}(\tau)$ denote the $\tau$-th quantile of $\ourvi$, that is, $\mathbb{P}(\widehat{\ourvi} \leq Q_{\widehat{\ourvi}}(\tau) ) = \tau$ and $\mathbb{P}(\ourvi \leq Q_{\ourvi}(\tau) ) = \tau$. Finally, let $\tau_{\text{low}} := t_{\text{low}} - 2\varepsilon_H$ and $\tau_{\text{up}} := t_{\text{up}} + 2\varepsilon_H$. Theorem \ref{thm:rid_finite_sample} states that, with $B \geq \frac{1}{2\varepsilon_H^2}\ln\left( \frac{2}{\delta} \right)$ bootstrap iterations, the following holds:
    \begin{align*}
        \mathbb{P}\left(\left| \mathbb{P}(\widehat{\ourvi} \leq k ) - \mathbb{P}(\ourvi \leq k )\right| \leq \varepsilon_H \right) \geq 1 -\delta,
    \end{align*}
    which implies the following looser bounds:
    \begin{align}
        &\mathbb{P}\left( \mathbb{P}(\ourvi \leq k ) - \mathbb{P}(\widehat{\ourvi} \leq k ) \leq \varepsilon_H  \right) \geq 1 -\delta
    \label{eq:rid-sub-est}
    \end{align}
    and
    \begin{align}
        &\mathbb{P}\left( \mathbb{P}(\widehat{\ourvi} \leq k )  - \mathbb{P}(\ourvi \leq k )\leq \varepsilon_H  \right) \geq 1 -\delta.
    \label{eq:est-sub-rid}
    \end{align}
    By Equation (\ref{eq:rid-sub-est}), we know that the probability of the following event is at least $1-\delta$:
    \begin{align*}
        & \mathbb{P}(\ourvi \leq Q_{\widehat{\ourvi}}(\tau_{\text{low}}) ) - \mathbb{P}\left(\widehat{\ourvi} \leq Q_{\widehat{\ourvi}}(\tau_{\text{low}}) \right) \leq \varepsilon_H  &\text{by setting $k = Q_{\widehat{\ourvi}}(\tau_{low})$}\\
        & \iff  \mathbb{P}\left[\ourvi \leq Q_{\widehat{\ourvi}}(\tau_{\text{low}}) \right] \leq \varepsilon_H + \mathbb{P}\left[\widehat{\ourvi} \leq Q_{\widehat{\ourvi}}(\tau_{\text{low}}) \right] \\
        & \iff \mathbb{P}\left[\ourvi \leq Q_{\widehat{\ourvi}}(\tau_{\text{low}}) \right] \leq \varepsilon_H + t_{\text{low}} - 2 \varepsilon_H  &\text{ b.c. $\mathbb{P}[\widehat{\ourvi} \leq Q_{\widehat{\ourvi}}(\tau_{\text{low}})] = t_{\text{low}} - 2 \varepsilon_H $ by definition}\\
        & \iff \mathbb{P}\left[\ourvi \leq Q_{\widehat{\ourvi}}(\tau_{\text{low}}) \right] \leq t_{\text{low}} - \varepsilon_H\\
    \end{align*}
    This states that, with high probability, the $\tau_{\text{low}}$ quantile of the distribution of $\widehat{\ourvi}$ is below the $t_{\text{low}} - \varepsilon_H$ quantile of $\ourvi$. We would like to explicitly draw a connection between some quantile of $\ourvi$ and $\widehat{\ourvi}$. To do so, we can then find the probability of the converse of the above as:
    \begin{align*}
        &\mathbb{P}\left[\mathbb{P}\left(\ourvi \leq Q_{\widehat{\ourvi}}(\tau_{\text{low}}) \right) \leq t_{\text{low}} - \varepsilon_H\right] \geq 1 - \delta \\
        & \iff 1 - \mathbb{P}\left[ \mathbb{P}\left(\ourvi \leq Q_{\widehat{\ourvi}}(\tau_{\text{low}}) \right) \leq t_{\text{low}} - \varepsilon_H\right] \leq \delta\\
        & \iff \mathbb{P}\left[ \mathbb{P}\left(\ourvi \leq Q_{\widehat{\ourvi}}(\tau_{\text{low}}) \right) > t_{\text{low}} - \varepsilon_H\right] \leq \delta\\
        & \iff \mathbb{P}\left[ \mathbb{P}\left(\ourvi \leq Q_{\widehat{\ourvi}}(\tau_{\text{low}}) \right) >  \mathbb{P}\left(\ourvi \leq Q_{\ourvi}(t_{\text{low}}) \right) - \varepsilon_H\right] \leq \delta &\text{ $t_{\text{low}} = \mathbb{P}\left(\ourvi \leq Q_{\ourvi}(t_{\text{low}})\right)$ by definition}\\
    \end{align*}
    %In other words, $Q_{\ourvi}(t_{\text{low}})$ is likely no more than $\varepsilon_H$ below $Q_{\widehat{\ourvi}}(\tau_{\text{low}})$. 
    
    We now use the above result to draw a connection between the (unknown) quantity $\mathbb{P}(\ourvi \leq Q_{\ourvi}(t_{\text{low}}) )$ and the (known) quantity $\mathbb{P}(\widehat{\ourvi} \leq Q_{\widehat{\ourvi}}(\tau_{\text{low}}) )$ by reintroducing the converse of Equation (\ref{eq:est-sub-rid}). From above,
    \begin{align*}
        &  \mathbb{P}\left[ \mathbb{P}\left(\ourvi \leq Q_{\widehat{\ourvi}}(\tau_{\text{low}}) \right) > \mathbb{P}\left(\ourvi \leq Q_{\ourvi}(t_{\text{low}}) \right) - \varepsilon_H\right] \leq \delta\\\\
        \iff &\mathbb{P}\left[ \mathbb{P}\left(\ourvi \leq Q_{\widehat{\ourvi}}(\tau_{\text{low}}) \right) >  \mathbb{P}\left(\ourvi \leq Q_{\ourvi}(t_{\text{low}}) \right) - \varepsilon_H\right] \\
        &+
        \mathbb{P}\left[\mathbb{P}\left(\widehat{\ourvi} \leq Q_{\widehat{\ourvi}}(\tau_{\text{low}}) \right) - \mathbb{P}\left(\ourvi \leq Q_{\widehat{\ourvi}}(\tau_{\text{low}})\right) \geq \varepsilon_H  \right]
        \leq \delta + \delta 
        &\text{By Equation (\ref{eq:est-sub-rid})}\\ \\
        \iff &\mathbb{P}\left[ \underbrace{\varepsilon_H + \mathbb{P}(\ourvi \leq Q_{\widehat{\ourvi}}(\tau_{\text{low}}) ) >  \mathbb{P}(\ourvi \leq Q_{\ourvi}(t_{\text{low}}) )}_{X} \right] \\
        &+
        \mathbb{P}\left[\underbrace{\mathbb{P}(\widehat{\ourvi} \leq Q_{\widehat{\ourvi}}(\tau_{\text{low}}) ) \geq \varepsilon_H + \mathbb{P}(\ourvi \leq Q_{\widehat{\ourvi}}(\tau_{\text{low}}))}_{Y} \right]
        \leq 2 \delta\\\\
        \implies &\mathbb{P}\Bigg[\left\{ \varepsilon_H + \mathbb{P}(\ourvi \leq Q_{\widehat{\ourvi}}(\tau_{\text{low}}) ) >  \mathbb{P}(\ourvi \leq Q_{\ourvi}(t_{\text{low}}) ) \right\} \\
        &\cup
        \left\{\mathbb{P}(\widehat{\ourvi} \leq Q_{\widehat{\ourvi}}(\tau_{\text{low}}) ) \geq \varepsilon_H + \mathbb{P}(\ourvi \leq Q_{\widehat{\ourvi}}(\tau_{\text{low}}))  \right\}\Bigg]
        \leq 2 \delta 
        &\text{By the Union Bound; since } \\
        &&\mathbb{P}(X \cup Y) \leq \mathbb{P}(X) + \mathbb{P}(Y) \leq 2\delta.
    \end{align*}
    This states that either (1) there is a small probability that $Q_{\widehat{\ourvi}}(\tau_{\text{low}})$ is larger than $Q_{\ourvi}(\tau_{\text{low}})$ or (2) there is a small probability that our estimate for $\ourvi$ at $Q_{\widehat{\ourvi}}(\tau_{\text{low}})$ is too large. We now invert this probability to show that, with high probability, $\mathbb{P}(\widehat{\ourvi} \leq Q_{\widehat{\ourvi}}(\tau_{\text{low}}) )$ provides a lower bound on $ \mathbb{P}(\ourvi \leq Q_{\ourvi}(t_{\text{low}}) ) $:
    \begin{align*}
        &\mathbb{P}\bigg[\left\{ \varepsilon_H + \mathbb{P}(\ourvi \leq Q_{\widehat{\ourvi}}(\tau_{\text{low}}) ) >  \mathbb{P}(\ourvi \leq Q_{\ourvi}(t_{\text{low}}) ) \right\} \\
        &\cup
        \left\{\mathbb{P}(\widehat{\ourvi} \leq Q_{\widehat{\ourvi}}(\tau_{\text{low}}) ) \geq \varepsilon_H + \mathbb{P}(\ourvi \leq Q_{\widehat{\ourvi}}(\tau_{\text{low}}))  \right\}\bigg]
        \leq 2 \delta\\
        \iff  & 1 - \mathbb{P}\bigg[\left\{ \varepsilon_H + \mathbb{P}(\ourvi \leq Q_{\widehat{\ourvi}}(\tau_{\text{low}}) ) > \mathbb{P}(\ourvi \leq Q_{\ourvi}(t_{\text{low}}) ) \right\} \\
        &\cup
        \left\{\mathbb{P}(\widehat{\ourvi} \leq Q_{\widehat{\ourvi}}(\tau_{\text{low}}) ) \geq \varepsilon_H + \mathbb{P}(\ourvi \leq Q_{\widehat{\ourvi}}(\tau_{\text{low}}))  \right\}\bigg]
        \geq 1 - 2 \delta\\
        \iff & \mathbb{P}\bigg[\left\{ \varepsilon_H + \mathbb{P}(\ourvi \leq Q_{\widehat{\ourvi}}(\tau_{\text{low}}) ) \leq \mathbb{P}(\ourvi \leq Q_{\ourvi}(t_{\text{low}}) ) \right\} \\
        &\cap
        \left\{\mathbb{P}(\widehat{\ourvi} \leq Q_{\widehat{\ourvi}}(\tau_{\text{low}}) ) < \varepsilon_H + \mathbb{P}(\ourvi \leq Q_{\widehat{\ourvi}}(\tau_{\text{low}}))  \right\}\bigg]
        \geq 1 - 2 \delta
        \end{align*}
    Since the term $\varepsilon_H + \mathbb{P}(\ourvi \leq Q_{\widehat{\ourvi}}(\tau_{\text{low}}))$ appears in both of the interior inequalities above, we can simplify the intersection by combining the two inequalities:
        \begin{align*}
        \mathbb{P}\bigg[&\left\{ \varepsilon_H + \mathbb{P}(\ourvi \leq Q_{\widehat{\ourvi}}(\tau_{\text{low}}) ) \leq \mathbb{P}(\ourvi \leq Q_{\ourvi}(t_{\text{low}}) ) \right\} \\
        &\cap
        \left\{\mathbb{P}(\widehat{\ourvi} \leq Q_{\widehat{\ourvi}}(\tau_{\text{low}}) ) < \varepsilon_H + \mathbb{P}(\ourvi \leq Q_{\widehat{\ourvi}}(\tau_{\text{low}}))  \right\}\bigg]
        \geq 1 - 2 \delta\\
        \iff & \mathbb{P}\left(\mathbb{P}(\widehat{\ourvi} \leq Q_{\widehat{\ourvi}}(\tau_{\text{low}}) ) < \varepsilon_H + \mathbb{P}(\ourvi \leq Q_{\widehat{\ourvi}}(\tau_{\text{low}}) ) \leq \mathbb{P}(\ourvi \leq Q_{\ourvi}(t_{\text{low}}) ) \right)
        \geq 1 - 2 \delta\\
        \iff & \mathbb{P}\left(\mathbb{P}(\widehat{\ourvi} \leq Q_{\widehat{\ourvi}}(\tau_{\text{low}}) ) < \mathbb{P}(\ourvi \leq Q_{\ourvi}(t_{\text{low}}) ) \right)
        \geq 1 - 2 \delta\\
        \iff & \mathbb{P}\left(\mathbb{P}(\widehat{\ourvi} \leq Q_{\widehat{\ourvi}}(\tau_{\text{low}}) ) \geq \mathbb{P}(\ourvi \leq Q_{\ourvi}(t_{\text{low}}) ) \right)
        \leq 2 \delta
    \end{align*}
    
    In other words, it is likely that the $\tau_{\text{low}}$-th quantile of $\widehat{\ourvi}$ provides a lower bound on the $t_{\text{low}}$-th quantile of $\ourvi$. 
    
    By following the same structure, we can derive a similar upper bound on the $t_{\text{up}}$-th quantile of $\ourvi$ in terms of $\widehat{\ourvi}$, arriving at the following result:
    \begin{align*}
        \mathbb{P}\left(\mathbb{P}(\widehat{\ourvi} \leq Q_{\widehat{\ourvi}}(\tau_{\text{up}}) ) \leq \mathbb{P}(\ourvi \leq Q_{\ourvi}(t_{\text{up}}) ) \right)
        \leq 2 \delta
    \end{align*}

    Finally, we can combine the upper and lower bounds we found above to find the probability that the $\epsilon ECR$ contains the desired $CCR$ as follows:
    \begin{align*}
        & \mathbb{P}\left(\mathbb{P}(\widehat{\ourvi} \leq Q_{\widehat{\ourvi}}(\tau_{\text{low}}) ) \geq \mathbb{P}(\ourvi \leq Q_{\ourvi}(t_{\text{low}}) ) \right) \\
        &+ \mathbb{P}\left(\mathbb{P}(\widehat{\ourvi} \leq Q_{\widehat{\ourvi}}(\tau_{\text{up}}) ) \leq \mathbb{P}(\ourvi \leq Q_{\ourvi}(t_{\text{up}}) ) \right) 
        \leq 2 \delta + 2 \delta\\
        \implies &\mathbb{P}\Bigg[\left\{\mathbb{P}(\widehat{\ourvi} \leq Q_{\widehat{\ourvi}}(\tau_{\text{low}}) ) \geq \mathbb{P}(\ourvi \leq Q_{\ourvi}(t_{\text{low}}) ) \right\} \\
        &\cup \left\{\mathbb{P}(\widehat{\ourvi} \leq Q_{\widehat{\ourvi}}(\tau_{\text{up}}) ) \leq \mathbb{P}(\ourvi \leq Q_{\ourvi}(t_{\text{up}}) ) \right\} \Bigg]
        \leq 4\delta
    \end{align*}
    We can then find a bound on $\mathbb{P}(CCR \subset ECR) = \mathbb{P}(\{ECR_{lb} \leq CCR_{lb}\} \cap \{ECR_{ub} \geq CCR_{ub}\})$ where $lb$ and $ub$ respectively denote the upper and lower bounds of their intervals they index, as: 
    \begin{align*}
        \mathbb{P}\Bigg(&\left\{\mathbb{P}(\widehat{\ourvi} \leq Q_{\widehat{\ourvi}}(\tau_{\text{low}}) ) \geq \mathbb{P}(\ourvi \leq Q_{\ourvi}(t_{\text{low}}) ) \right\} \\
        &\cup \left\{\mathbb{P}(\widehat{\ourvi} \leq Q_{\widehat{\ourvi}}(\tau_{\text{up}}) ) \leq \mathbb{P}(\ourvi \leq Q_{\ourvi}(t_{\text{up}}) ) \right\} \Bigg)
        \leq 4\delta\\
        \iff & 1 - \mathbb{P}\bigg(\left\{\mathbb{P}(\widehat{\ourvi} \leq Q_{\widehat{\ourvi}}(\tau_{\text{low}}) ) \geq \mathbb{P}(\ourvi \leq Q_{\ourvi}(t_{\text{low}}) ) \right\} \\
        &\cup \left\{\mathbb{P}(\widehat{\ourvi} \leq Q_{\widehat{\ourvi}}(\tau_{\text{up}}) ) \leq \mathbb{P}(\ourvi \leq Q_{\ourvi}(t_{\text{up}}) ) \right\} \bigg)
        \geq 1 - 4\delta\\
        \iff &\mathbb{P}\bigg(\left\{\mathbb{P}(\widehat{\ourvi} \leq Q_{\widehat{\ourvi}}(\tau_{\text{low}}) ) < \mathbb{P}(\ourvi \leq Q_{\ourvi}(t_{\text{low}}) ) \right\} \\
        &\cap \left\{\mathbb{P}(\widehat{\ourvi} \leq Q_{\widehat{\ourvi}}(\tau_{\text{up}}) ) > \mathbb{P}(\ourvi \leq Q_{\ourvi}(t_{\text{up}}) ) \right\} \bigg)
        \geq 1 - 4\delta\\
        \iff &\mathbb{P} \bigg( \big(\mathbb{P}(\ourvi \leq Q_{\ourvi}(t_{\text{low}}) ), \mathbb{P}(\ourvi \leq Q_{\ourvi}(t_{\text{up}}) )\big)\\
        &\subset \left(\mathbb{P}(\widehat{\ourvi} \leq Q_{\widehat{\ourvi}}(\tau_{\text{low}}) ), \mathbb{P}(\widehat{\ourvi} \leq Q_{\widehat{\ourvi}}(\tau_{\text{up}}) )\right) \bigg)
        \geq 1 - 4\delta\\
        \iff &\mathbb{P}(CCR \subset ECR) \geq 1 - 4\delta \\
    \end{align*}
    With high probability, this states that the region of $\ourvi$ between $t_{\text{low}}$ and $t_{\text{up}}$ is contained within the region of $\widehat{\ourvi}$ between $\tau_\text{low}$ and $\tau_\text{up}$ with $B \geq \frac{1}{2\varepsilon_H^2}\ln\left( \frac{2}{\delta} \right)$ bootstrap iterations. This can be equivalently stated as
    \begin{align*}
        &\mathbb{P}(CCR \subset ECR) \geq
         1 - \delta
    \end{align*}
    with $B \geq \frac{1}{2\varepsilon_H^2}\ln\left( \frac{8}{\delta} \right)$ bootstrap iterations.
    
\end{proof}
