# Supplementary material for: The Rashomon Importance Distribution: Getting RID of Unstable, Single Model-based Variable Importance
Source: arXiv:2309.13775 source file (2024-04-01)
Supplement: Supplementary file 2 [file rashomon_stability.tex]

\begin{theorem}
    Let $\mathcal{P}_n, \mathcal{P}_n'$ represent the empirical density functions for datasets $\Dn_1, \Dn_2$ sampled i.i.d. from the same data generating process. 
    
    Let $\delta = \| \mathcal{P}_n - \mathcal{P}_n' \|_{\infty} = \sup_z |\mathcal{P}_n(z) - \mathcal{P}_n'(z)|.$ Let $\mathbf{k} \in [\phi_{min}, \phi_{max}]^p$ As $\delta$ decreases, the distance between the JRID following $\mathcal{P}_n$ and the JRID following $\mathcal{P}_n'$ decreases:
    
    \begin{align*}
        \text{ As } \delta \text{ decreases },
        \left|F_{JRID \sim \mathcal{P}_n}\left(\mathbf{k}\right) - F_{JRID \sim \mathcal{P}_n'}\left(\mathbf{k}\right) \right| 
    \end{align*}
    also decreases.
\end{theorem}

\begin{proof}
    Let $\mathcal{P}_n, \mathcal{P}_n', \mathcal{P}_n''$ represent the empirical density functions for datasets $\Dn_1, \Dn_2, \Dn_3$ sampled i.i.d. from the same data generating process. 
    
    Let $\delta_1 = \| \mathcal{P}_n - \mathcal{P}_n' \|_{\infty} = \sup_z |\mathcal{P}_n(z) - \mathcal{P}_n'(z)|$ and let $\delta_2 = \| \mathcal{P}_n - \mathcal{P}_n'' \|_{\infty} = \sup_z |\mathcal{P}_n(z) - \mathcal{P}_n''(z)|.$ Assume $\delta_1 < \delta_2.$ In other words, assume the empirical distribution $\mathcal{P}_n$ is closer to $\mathcal{P}_n'$ than it is to $\mathcal{P}_n''.$

    First, recognize that
    \begin{align*}
        F_{JRID \sim \mathcal{P}_n}\left(\mathbf{k}\right) 
        &= 
        \mathbb{E}_{\Dn \sim \mathcal{P}_n}\left[ \frac{\sum_{f \in \mathcal{R}_{\Dn}^\varepsilon} \mathbb{1}\left[\phi(f, \Dn) \leq \mathbf{k}  \right]}{|\mathcal{R}_{\Dn}^\varepsilon|} \right] \\
        &= \mathbb{E}_{\Dn \sim \mathcal{P}_n}\left[ \frac{\sum_{f \in \mathcal{R}_{\Dn}^\varepsilon} \mathbb{1}\left[\phi(f, \Dn) \leq \mathbf{k}  \right]}{|\mathcal{R}_{\Dn}^\varepsilon|} \right] \\
        &= \int_{\Dn} \left[ \frac{\sum_{f \in \mathcal{R}_{\Dn}^\varepsilon} \mathbb{1}\left[\phi(f, \Dn) \leq \mathbf{k}  \right]}{|\mathcal{R}_{\Dn}^\varepsilon|} \right] \mathcal{P}_n(\Dn) d\Dn,
    \end{align*}
    where $\int_{\Dn} d\Dn$ represents the integral over all possible datasets that could be generated from $\mathcal{P}_n$; in the case of discrete datasets, the proof still holds by replacing $\int_{\Dn} d\Dn$ with a summation over all possible $\Dn \sim \mathcal{P}_n.$ Additionally, $\mathcal{P}_n(\Dn)$ represents the density associated with observing the dataset $\Dn.$

    Now, we can represent $\left|F_{JRID \sim \mathcal{P}_n}\left(\mathbf{k}\right) - F_{JRID \sim \mathcal{P}_n'}\left(\mathbf{k}\right) \right|$ in terms of $\delta_1$

     \begin{align*}
         &\left|F_{JRID \sim \mathcal{P}_n}\left(\mathbf{k}\right) - F_{JRID \sim \mathcal{P}_n'}\left(\mathbf{k}\right) \right| \\
         = & \left| \int_{\Dn} \left[ \frac{\sum_{f \in \mathcal{R}_{\Dn}^\varepsilon} \mathbb{1}\left[\phi(f, \Dn) \leq \mathbf{k}  \right]}{|\mathcal{R}_{\Dn}^\varepsilon|} \right] \mathcal{P}_n(\Dn) d\Dn -  \int_{\Dn} \left[ \frac{\sum_{f \in \mathcal{R}_{\Dn}^\varepsilon} \mathbb{1}\left[\phi(f, \Dn) \leq \mathbf{k}  \right]}{|\mathcal{R}_{\Dn}^\varepsilon|} \right] \mathcal{P}_n'(\Dn) d\Dn \right| \\
         = & \left| \int_{\Dn} \left[ \frac{\sum_{f \in \mathcal{R}_{\Dn}^\varepsilon} \mathbb{1}\left[\phi(f, \Dn) \leq \mathbf{k}  \right]}{|\mathcal{R}_{\Dn}^\varepsilon|} \right] \mathcal{P}_n(\Dn) d\Dn -  \int_{\Dn} \left[ \frac{\sum_{f \in \mathcal{R}_{\Dn}^\varepsilon} \mathbb{1}\left[\phi(f, \Dn) \leq \mathbf{k}  \right]}{|\mathcal{R}_{\Dn}^\varepsilon|} \right] \mathcal{P}_n'(\Dn) d\Dn \right| \\
         = &\left| \int_{\Dn} \left[ \frac{\sum_{f \in \mathcal{R}_{\Dn}^\varepsilon} \mathbb{1}\left[\phi(f, \Dn) \leq \mathbf{k}  \right]}{|\mathcal{R}_{\Dn}^\varepsilon|} \right] \left(\mathcal{P}_n(\Dn) - \mathcal{P}_n'(\Dn) \right) d\Dn \right| \\
         = &\left| \int_{\Dn} \left[ \frac{\sum_{f \in \mathcal{R}_{\Dn}^\varepsilon} \mathbb{1}\left[\phi(f, \Dn) \leq \mathbf{k}  \right]}{|\mathcal{R}_{\Dn}^\varepsilon|} \right] \left(\mathcal{P}_n(\Dn) - \mathcal{P}_n'(\Dn) \right) d\Dn \right| \\
         \leq &\int_{\Dn} \left| \left[ \frac{\sum_{f \in \mathcal{R}_{\Dn}^\varepsilon} \mathbb{1}\left[\phi(f, \Dn) \leq \mathbf{k}  \right]}{|\mathcal{R}_{\Dn}^\varepsilon|} \right] \left(\mathcal{P}_n(\Dn) - \mathcal{P}_n'(\Dn) \right) \right| d\Dn \text{ by Triangle Ineq. } \\
         = &\int_{\Dn} \underbrace{\left[ \frac{\sum_{f \in \mathcal{R}_{\Dn}^\varepsilon} \mathbb{1}\left[\phi(f, \Dn) \leq \mathbf{k}  \right]}{|\mathcal{R}_{\Dn}^\varepsilon|} \right]}_{(*)} \left|  \left(\mathcal{P}_n(\Dn) - \mathcal{P}_n'(\Dn) \right) \right| d\Dn \text{ because } 0 \leq (*) \leq 1 \\
         < &\int_{\Dn} \underbrace{\left[ \frac{\sum_{f \in \mathcal{R}_{\Dn}^\varepsilon} \mathbb{1}\left[\phi(f, \Dn) \leq \mathbf{k}  \right]}{|\mathcal{R}_{\Dn}^\varepsilon|} \right]}_{(*)} \left|  \left(\mathcal{P}_n(\Dn) - \mathcal{P}_n''(\Dn) \right) \right| d\Dn \text{ because } 
         &
     \end{align*}
    
\end{proof}
